# Supplementary material for: A Survey on Cloud-Edge-Terminal Collaborative Intelligence in AIoT Networks
Source: arXiv:2508.18803 source file (2026-11-15)
Supplement: Supplementary file 1 [file supp.pdf]

# *Supplementary Material*
# A Survey on Cloud-Edge-Terminal Collaborative Intelligence in AIoT Networks

Jiaqi Wu, Jing Liu, Yang Liu, *Member, IEEE*, Lixu Wang, Zehua Wang, *Member, IEEE*, Wei Chen, *Member, IEEE*, Zijian Tian, F. Richard Yu, *Fellow, IEEE*, Victor C.M. Leung, *Life Fellow, IEEE*

## I. Overview

In this supplementary material, we provide more detailed coverage of key cloud-edge-terminal collaborative intelligence (CETCI) components that are not fully addressed in the main paper due to page limitations. We have moved comprehensive explanations of 1) optimization techniques for task offloading and resource allocation, 2) security mechanisms and privacy-preserving techniques, 3) data management and communication protocols, and 4) specific application domains to this supplement. Specifically, Sec. III covers mathematical and learning-based optimization techniques including linear programming, convex optimization, and game theory approaches. Sec. IV presents detailed security mechanisms and privacy-preserving techniques for collaborative intelligence systems. Sec. II provides comprehensive analysis of data management and communication protocols in distributed AIoT environments. Sec. V showcases specific applications in smart cities and smart agriculture domains, demonstrating the practical implementation of cloud-edge-terminal collaboration.

## II. Optimization Techniques in Intelligent Resource Management

Mathematical and learning-based optimization approaches address the complex challenges of task offloading and resource allocation in distributed computing environments. This section provides detailed coverage of three fundamental optimization paradigms: linear programming, convex optimization, and game theory. Each approach offers unique advantages for solving resource management problems in cloud-edge-terminal collaborative systems. Table I summarizes representative optimization techniques across different algorithm types and scenarios, demonstrating their performance improvements in metrics such as response time, latency, and energy consumption.

### A. Linear Programming

Constrained optimization under linear relationships enables tractable solutions for resource allocation problems. LP formulations transform complex distribution challenges into mathematically solvable frameworks with guaranteed optimal solutions [28]. For example, the objective function might minimize total system cost, encompassing energy consumption at terminal and edge layers [29], computation costs at the

TABLE I: Summary of optimization techniques.

| Method | Year | Venue | Algorithm Type | Scenarios | Performance Metrics | Performance Results |
|---|---|---|---|---|---|---|
| TIGO [1] | 2024 | IEEE TSC | Two-stage Iterated Greedy Optimization | Cloud-Edge Collaborative Computing | Average Response Time | Better response times in less time compared to existing methods |
| DSCF [2] | 2024 | IEEE IoTJ | CMDP-based Framework | Distributed Serverless Edge Clouds | Inference Latency | Less than half the inference latency compared to local computing |
| AWSH [3] | 2024 | IEEE TMC | Hyper-Heuristic Algorithm | 5G Mobile Edge Clouds | Latency, Load Balancing | Superior performance compared to SOTA solutions |
| Lu et al. [4] | 2024 | IEEE TVT | Multi-Agent Reinforcement Learning | IoV Edge Cloud | Quality of Service | Effective performance in complex network situations |
| Nguyen et al. [5] | 2024 | IEEE TCC | Alternating Optimization | Space-Air-Ground Networks | Energy Consumption, Delay | Superior effectiveness compared to baselines |
| Qiu et al. [6] | 2024 | IEEE TMC | Online Algorithm | Edge Intelligence Cloud | Security, Reliability, Throughput | Promising performance compared to baseline algorithms |
| Wei et al. [7] | 2024 | IEEE TPDS | Two-stage Algorithm | Federated Learning in Edge Clouds | Learning Costs | 33.5%-39.6% lower average total costs vs. previous methods |
| SemCom-SEC [8] | 2024 | IEEE JSAC | Federated Learning, Game Theory | Satellite-Borne Edge Cloud Network | Delay, Energy Consumption, Privacy | Reduced delay and energy consumption while enhancing privacy |
| Asgarian et al. [9] | 2024 | IEEE IoTJ | Approximation Algorithm | Edge-Cloud Computing Industrial IoT | Delay, Resource Consumption | Near-optimal solution with polynomial time complexity |
| Bai et al. [10] | 2024 | IEEE TMC | Convex Approximation, Lyapunov Optimization | UAV-Enabled Edge-Cloud Computing | Task Completion Delay | Significant reduction in task completion delay |
| JTOCC [11] | 2024 | IEEE TWC | DRL, LSTM | NOMA-Aided CETCI | Network Latency | Lower-delay content distribution and fast convergence |
| PRAISE [12] | 2024 | IEEE TMC | Task Reconfiguration | Multi-Access Edge Cloud Networks | Total Offloading Benefit | Higher system benefits and lower resource costs than baselines |
| CORA [13] | 2024 | IEEE TWC | Data-driven Optimization | Mobile Edge Clouds | Quality of Experience | 18% reduction in user complaint rate on YouTube dataset |
| Co-NOMA [14] | 2024 | IEEE IoTJ | Cooperative NOMA | Reality in Cloud/Edge Computing | Logarithmic Rate, Delay | Outperforms traditional multiple access and NOMA methods |
| Xiao et al. [15] | 2024 | IEEE IoTJ | Online Learning | Video Caching in IoT Networks | Delay, Resource Utilization | Performance advantages compared to SOTA algorithms |
| ADMM-FedMeta [16] | 2021 | MobiHoc | Federated Meta-Learning | Edge Learning in IoT | Learning Performance, Computational Cost | Substantially outperforms existing baselines |
| RL-ROIS [17] | 2024 | IEEE IoTJ | Reinforcement Learning | RIS-Aided IoT Networks | Capacity, Latency, Energy Consumption | Superior efficiency and robustness |
| Zhao et al. [18] | 2024 | IEEE TMC | Online Algorithm | Serverless Cloud Inference | Inference Latency, Cost, Accuracy | Less than half inference latency compared to local computing |
| MESP [19] | 2024 | IEEE IoTJ | Game Theory | Industry 5.0 | End-to-End Execution Delay | 20%-30% reduction in computational overhead and delay |
| COMEC [20] | 2024 | IEEE TMC | Algorithm | Multi-Cell Networks | Total cost (delay and energy) | Superior system cost compared to baselines |
| Zhou et al. [21] | 2024 | ADHOC | Framework | AIoT | Quality of Service | Higher effectiveness and efficiency than centralized approach |
| Dragotto et al. [22] | 2024 | JCC | Game-theoretic model | Cloud Networks | Network security posture | Efficacy demonstrated through computational tests |
| Raj et al. [23] | 2021 | ArXiv | Framework | Edge IoT | Efficiency, Robustness | Validated through air quality forecasting experiment |
| PGRA [24] | 2020 | ArXiv | Algorithm | Satellite Edge Computing | Network payoff, Deployment cost | Effectively addresses VNF placement problem |
| MADRLOM [25] | 2024 | COMNET | Mechanism | Software-Defined Cloud-Edge Networks | System overhead | Significant reduction in total system overhead |
| Zhang et al. [26] | 2024 | IEEE TCC | Game-theoretic | Mobile Edge Computing | Task completion delay, User cost | Superior performance compared to several approaches |
| Li et al. [27] | 2024 | ArXiv | Framework | Wireless Powered Edge Computing | Weighted sum computation rate | Comparable to exhaustive search with reduced execution time |

cloud and edge [1], and network communication costs [5]. Constraints can represent resource limitations, such as bandwidth [30], processing capacity at each layer [31], and latency [3]. LP also supports various task offloading strategies, including decisions on offloading locations (edge or cloud) and resource allocation [6]. Additionally, incorporating predicted future system states into the LP formulation enables proactive resource management in dynamic AIoT environments [4].

### B. Convex Optimization

Nonlinear optimization with convergence guarantees addresses complex resource distribution challenges. Convex programming techniques enable globally optimal solutions through gradient-based methods and interior-point algorithms [5]. As an example, resource allocation might aim to minimize energy consumption under latency and throughput constraints. If these constraints and the objective function are convex, gradient descent can iteratively update resource allocation based on the objective function's gradient, while interior-point methods traverse the feasible region for optimal solutions [12]. Several studies have explored this approach, including [32], which uses online convex optimization for network slicing in edge-cloud orchestrated networks to minimize system costs. Similarly, [33] employs convex optimization for resource and power allocation in cloud-edge collaboration to minimize user overhead. In addition, [11] uses successive convex approximation (SCA) for resource optimization in NOMA-aided cloud-edge-terminal cooperation, and [10] applies convex approximation to a delay minimization problem in multi-UAV enabled edge-cloud cooperation. However, formulating such convex programs often requires simplifications to address the complexity and dynamic nature of cloud-edge-terminal environments.

### C. Game Theory

Competitive and cooperative interaction modeling provides equilibrium-based optimization frameworks. Strategic decision-making among rational participants enables stable resource allocation through concepts like Nash equilibrium and Stackelberg leadership [34]. For instance, [20] formulates a non-cooperative game for distributed cost minimization in multi-cell networks, demonstrating game theory's applicability to computation offloading in edge-cloud collaboration. Similarly, [26] uses a Stackelberg game to model user, base station, and cloud interactions in multi-user multi-task offloading for mobile edge computing. Beyond resource allocation, game theory also addresses security, as exemplified by [22], which introduces the critical node game for assessing cybersecurity risks in cloud networks. Additionally, [35] proposes a game-theoretic algorithm for optimizing system completion time and energy consumption in cloud robot task offloading. Cooperative solutions, such as the Nash bargaining solution in [36] for joint latency-energy minimization in fog-assisted networks, offer alternative approaches for various collaboration paradigms. For instance, examples, including task offloading [19], resource allocation [37], and collaborative computation [38], highlight game theory's utility in optimizing resource management for cloud-edge-terminal collaboration.

## III. Security Mechanisms and Privacy-Preserving Techniques

### A. Security Mechanisms and Solutions

Protecting collaborative intelligence paradigms against various threats requires robust security mechanisms. We explore three key security solutions: encryption and authentication, intrusion detection and prevention, and blockchain technologies. Encryption and authentication techniques safeguard data transmission and storage across distributed architectures. Additionally, intrusion detection and prevention systems proactively identify and mitigate security breaches. Finally, blockchain technologies offer potential enhancements to security and trust establishment within collaborative environments.

*1) Encryption and Authentication:* Cryptographic protection mechanisms secure data transmission and storage across distributed computing layers. Strong encryption protocols combined with robust authentication systems prevent unauthorized access while maintaining communication efficiency [39]. Lightweight symmetric encryption secures data exchange between resource-constrained devices and edge nodes, while CP-ABE [40] offers fine-grained access control based on specific criteria, addressing the varying data sensitivity in AIoT environments. Authentication verifies the identity of communicating entities, preventing unauthorized access and manipulation. For example, GS-SNC enhances security through scrambling and encoding, offering advantages in computational complexity and space overhead compared to other secure network coding approaches like DP-SNC and SPOC [41]. Integrating blockchain technology strengthens security by providing immutable records of data transactions and access logs [42], and homomorphic signatures enable efficient third-party integrity auditing without accessing raw data [43].

*2) Intrusion Detection and Prevention:* Proactive threat monitoring systems identify and neutralize malicious activities before system compromise. Real-time anomaly detection enables rapid response to security incidents across distributed computing infrastructure [21]. For example, unusual data flows between the edge and cloud, or sudden spikes in data transmission at the terminal layer, can signal intrusions [44]. Deploying IDPS at different architectural layers, such as the edge or cloud, provides comprehensive security coverage [45]. Edge-based IDPS enables faster responses to localized threats by analyzing data near the source, while cloud-based IDPS leverages centralized resources to identify complex attack patterns [42]. In addition to detection, IDPS [23] incorporates prevention mechanisms, including blocking malicious traffic and isolating compromised devices, to actively mitigate threats. Table II provides an overview of methods addressing security threats and vulnerabilities in collaborative intelligence systems, highlighting their deployment scenarios and performance metrics across different architectural configurations.

*3) Blockchain Technologies:* Decentralized trust mechanisms eliminate single points of failure while ensuring immutable transaction records. Distributed consensus protocols enhance system resilience and provide transparent, tamper-proof data management [53]. Cryptographic hashing and consensus mechanisms, integral to blockchain's architecture,

TABLE II: Summary of methods addressing security threats and vulnerabilities in CISAIOT networks.

| Method | Year | Venue | Scenarios | Performance Metrics | Edge | Cloud | ECC | CETC |
|---|---|---|---|---|---|---|---|---|
| Yang et al. [46] | 2024 | IEEE IoTJ | AIoT Data Prediction | Privacy and Accuracy | ✓ | ✓ | ✓ | ✓ |
| Rahman et al. [47] | 2023 | IEEE IoTJ | Industry 4.0 CPS | Security, Detection Performance | ✓ | ✓ | ✓ | ✗ |
| Fang et al. [41] | 2024 | IEEE IoTJ | CETC-AIoT | Computational Complexity | ✓ | ✓ | ✓ | ✓ |
| Chen et al. [48] | 2024 | IEEE TNSE | Workflow Scheduling | Execution Cost, Deadline Constraints | ✓ | ✓ | ✓ | ✗ |
| Wang et al. [49] | 2022 | ArXiv | Security Inference | Privacy-Utility Tradeoff | ✓ | ✓ | ✓ | ✗ |
| Zhou et al. [21] | 2024 | ADHOC | AIoT Services | QoS, Effectiveness, Efficiency | ✓ | ✓ | ✓ | ✗ |
| Wang et al. [50] | 2018 | ArXiv | IoT Security | Attack Detection | ✗ | ✗ | ✗ | ✗ |
| Li et al. [51] | 2022 | IEEE TII | Industrial IoT | Attack Cost, Detection Accuracy | ✓ | ✗ | ✓ | ✗ |
| Chi et al. [42] | 2024 | IEEE IoTJ | AIoT Edge Applications | Security, Model Efficiency | ✓ | ✓ | ✓ | ✓ |
| Raj et al. [23] | 2021 | ArXiv | AIoT Applications | Efficiency, Robustness | ✓ | ✓ | ✓ | ✗ |
| Dui et al. [52] | 2024 | RESS | IIoT Systems | Reliability, Gateway Cost | ✓ | ✓ | ✓ | ✗ |
| Xiao et al. [40] | 2024 | IEEE TIFS | Cloud-Edge IoT | Security, Efficiency | ✓ | ✓ | ✓ | ✓ |

ensure data integrity and prevent unauthorized tampering [47], which is crucial for secure data aggregation and processing from numerous AIoT devices. Furthermore, blockchain facilitates secure access control and device authentication within the collaborative ecosystem [42]. Through smart contracts, predefined rules and policies are automatically enforced, streamlining device interactions and ensuring compliance for activities such as sensitive data access and resource allocation across the cloud, edge, and terminal layers [54]. Applications of blockchain integration in AIoT include secure data logging and auditing, decentralized avionics services, and trusted decision architectures [55].

### B. Privacy-Preserving Techniques

Protecting user data within distributed collaborative systems is paramount. Four prominent techniques address privacy concerns: federated learning, differential privacy, homomorphic encryption, and secure multi-party computation. Federated learning enables collaborative model training without sharing raw data, while differential privacy adds noise to further protect individual data points. Homomorphic encryption allows computations on encrypted data without decryption, and secure multi-party computation enables joint computation on private inputs, revealing only the output.

*1) Federated Learning and Differential Privacy:* Complementary privacy mechanisms combine to strengthen distributed learning frameworks [56]. FL facilitates collaborative model training without direct data sharing [57], where edge devices or terminals train local models and share only model updates (e.g., gradients) with a central server [58]. However, potential information leakage from the updates necessitates further privacy enhancements through DP [59]. Specifically, DP introduces calibrated noise to these shared updates, ensuring that the presence or absence of a single data point does not significantly affect the final model [49], thereby hindering adversarial attempts to infer individual user data. Techniques like objective perturbation, adding noise to the objective function, achieve DP guarantees in FL [46]. The privacy-utility trade-off is controlled by the privacy budget ($\epsilon$, $\delta$), exemplified by differentially private over-the-air FL where transmit power adjustments influence this trade-off [60].

*2) Homomorphic Encryption:* Computational privacy through encrypted data processing eliminates decryption requirements during analysis [39, 60]. Beyond traditional cryptographic approaches, HE enables secure data aggregation, model training, and inference across distributed devices and cloud servers. For example, edge devices can encrypt sensor readings using HE before transmission, ensuring data confidentiality during transit and storage, even if intermediary nodes are compromised [61]. Consequently, cloud servers can perform computations on this encrypted data without decryption, enabling tasks like model training and inference on sensitive data [62]. In collaborative learning, HE facilitates secure model updates by enabling encrypted aggregation of model parameters [63]. Hierarchical federated learning frameworks demonstrate the practical integration of HE with multi-level privacy protection, exemplified by digital twin-based anomaly detection systems in smart healthcare that utilize edge cloudlets for local model training while preserving patient data privacy through encrypted multi-party collaboration [64]. Additionally, verifiable encodings and authenticators built upon HE can ensure the correctness of cloud-based computations on encrypted data [65]. Although the benefits are substantial, practical application of HE faces challenges related to computational overhead. However, ongoing research focuses on optimizing HE schemes, including using GPUs for accelerated computations and developing privacy-authority-aware compilers for efficient ciphertext management [66].

*3) Secure Multi-Party Computation:* Joint computation over private datasets maintains input confidentiality across participating entities [67]. Multiple parties—including cloud servers, edge nodes, and devices—can collaboratively compute functions over their combined data while preserving individual input secrecy, particularly crucial for sensitive information such as patient health records [21] or manufacturing process data [42]. For example, multiple hospitals could leverage MPC to train a shared machine learning model on patient data without directly sharing the raw data due to privacy regulations. Consequently, model updates can be jointly computed based on local datasets without revealing individual patient records. Similarly, MPC enhances security in task offloading and resource allocation within cooperative networks [41], facilitating collaborative decision-making regarding resource utilization without disclosing individual constraints or priorities. Furthermore, integrating MPC with techniques such as federated learning [46] and differential privacy [68] provides a more comprehensive privacy solution. For example, this integration enables secure aggregation of model updates or the addition of noise to computation outputs.

## IV. Data Management and Communication

### A. Data Storage and Retrieval

Efficient data management is crucial for collaborative intelligence in distributed systems. Edge caching plays a key role in optimizing data access and minimizing network congestion.

TABLE III: Summary of data preprocessing methods for efficient transmission in resource-constrained AIoT environments.

| Method | Year | Venue | Type | Scenarios | Performance Metrics | Edge | Cloud | ECC | CETC |
|---|---|---|---|---|---|---|---|---|---|
| Raj et al. [23] | 2021 | ArXiv | Edge MLOps | AIoT Fleet Analytics | Forecasting Accuracy | ✓ | ✓ | ✓ | ✗ |
| Becker et al. [69] | 2020 | IEEE BigData | AIOps | Edge Computing | Resource Utilization, Detection Performance | ✓ | ✓ | ✗ | ✗ |
| QuAsyncFL [58] | 2024 | IEEE IoTJ | Federated Learning | Cloud-Edge-Terminal AIoT | Communication Efficiency, Convergence | ✓ | ✓ | ✓ | ✓ |
| Underwood et al. [70] | 2024 | ArXiv | Data Compression | ML/AI Training | Compression Ratio, Model Quality | ✓ | ✓ | ✗ | ✗ |
| Noura et al. [71] | 2023 | Ad Hoc Netw. | DL-based Compression | Multimedia IoT | Visual Quality, Compression Ratio | ✓ | ✓ | ✓ | ✗ |
| Edge Source Coding [72] | 2019 | ArXiv | Lossless Compression | Edge Networks | Number of Bits Needed | ✓ | ✗ | ✗ | ✗ |
| Taurone et al. [73] | 2023 | ArXiv | Floating-point Compression | IoT Time-Series Data | Compression Ratio, Recovery Error | ✓ | ✗ | ✗ | ✗ |
| Shadura et al. [74] | 2020 | ArXiv | Lossless Compression | HEP Analysis | I/O Bandwidth, Storage Space | ✗ | ✓ | ✗ | ✗ |
| Melissaris et al. [75] | 2020 | ArXiv | Selective Compression | IoT and Web Traffic | Network Transfer Speed, Data Savings | ✓ | ✗ | ✗ | ✗ |
| Banerjee et al. [76] | 2022 | ArXiv | Hybrid Compression | Scientific Data | Compression Factor, QoI Preservation | ✓ | ✓ | ✓ | ✗ |
| LTSDC [77] | 2022 | ArXiv | Statistical Compression | IoT Time-Series Data | Compression Ratio | ✓ | ✗ | ✗ | ✗ |
| Zhou et al. [21] | 2024 | ADHOC | Federated Learning | Edge-Cloud AIoT | QoS, Latency | ✓ | ✓ | ✓ | ✗ |
| Arroba et al. [78] | 2023 | ArXiv | Sustainable Computing | Edge Infrastructure | Energy Efficiency | ✓ | ✓ | ✗ | ✗ |
| QOMVN [79] | 2024 | JCC | Edge Collaborative Caching | Vehicular Networks | Data Query Latency | ✓ | ✗ | ✓ | ✗ |
| Rac et al. [80] | 2021 | ArXiv | Containerization | Edge Computing | Application Execution Efficiency | ✓ | ✓ | ✗ | ✗ |

Furthermore, distributing data across cloud and edge nodes requires consideration of data consistency, availability, and access efficiency. Maintaining data integrity and ensuring high availability against potential disruptions and security threats also pose significant challenges in distributed environments. Table III presents a comprehensive overview of data management and communication techniques, categorizing methods by their deployment scenarios and key performance metrics such as latency reduction, throughput improvement, and reliability enhancement.

*1) Edge Caching:* Proximity-based storage strategies reduce access latency through intelligent content placement near end-users [81]. Popular data items stored at network edges increase cache hit rates and minimize retrieval delays. Result caching extends this concept by storing computation results, which is particularly advantageous for computationally intensive tasks [82]. Similarly, predictive caching anticipates future requests based on historical patterns and preemptively stores data, further minimizing latency [83, 84]. For example, PEC employs deep learning for content popularity prediction and prefetching [83], while a D3QN-based scheme dynamically evaluates content importance for efficient caching and eviction in dynamic networks [85]. In vehicular networks, edge collaborative caching, aided by tabu search algorithms, prioritizes high-traffic data and ensures backup within the collaborative domain to reduce latency and prevent single-point failures [79].

*2) Distributed Data Storage:* Multi-tier storage architectures enable efficient data distribution across cloud and edge infrastructures [86]. Proximity-based storage reduces latency for real-time applications while enhancing fault tolerance through geographical distribution [23]. Distributing data across multiple nodes enhances fault tolerance, ensuring system reliability even with individual node failures [42]. Strategic data placement, based on access patterns, caches frequently accessed data at the edge for faster retrieval, while less frequently used data resides in the cloud [69]. Data partitioning techniques divide large datasets into smaller chunks distributed across multiple nodes, facilitating parallel processing and improving system performance [46]. Additionally, essential data synchronization mechanisms maintain consistency and data integrity across distributed locations, preventing conflicts from concurrent updates [21]. Security considerations are addressed through encryption techniques for data confidentiality and access control mechanisms to restrict unauthorized access [27].

*3) Data Integrity and Availability:* Comprehensive protection mechanisms ensure information authenticity and continuous accessibility across distributed networks [52]. Trustworthy decision-making requires robust data integrity, exemplified by blockchain applications for enhanced security [42]. Addressing authentication and preventing model poisoning attacks, as discussed in [87] and [46], respectively, are also critical. Data availability, ensuring data accessibility, can be impacted by fluctuating resources and bandwidth in dynamic edge networks, especially for time-sensitive applications [88]. Efficient data storage and retrieval, including edge caching techniques [23], are thus essential for improving data access latency and enhancing availability. Similarly, distributed data storage across multiple nodes, as highlighted in the CEFIoT architecture [87], improves fault tolerance and resilience.

### *B. Communication Protocols and Optimization*

Efficient data exchange is crucial for distributed collaborative systems. We explore communication protocols and optimization techniques that enable effective data transmission. Established protocols like MQTT and CoAP enable efficient data transmission in complex environments. Furthermore, bandwidth optimization methods, including traffic scheduling, rate adaptation, and link aggregation, maximize data throughput and minimize latency. Additionally, fault tolerance mechanisms, such as error detection and recovery, connection management, and service monitoring, ensure reliable communication, contributing to overall performance and stability.

*1) Communication Protocols:* Resource-aware messaging protocols optimize data exchange efficiency in constrained CISAIOT environments. MQTT [89] and CoAP [90] exemplify lightweight approaches designed for low-overhead communication. MQTT, a publish-subscribe protocol with low overhead and diverse QoS levels, suits resource-constrained environments and various AIoT applications [91]. Open-source MQTT broker implementations, such as Mosquitto and EMQX, are readily available and have been experimentally benchmarked in edge computing [92]. CoAP, specifically designed for resource-constrained devices and networks, offers a RESTful interface for interaction with web services and has been explored with security mechanisms like OSCORE [90]. In addition, network coding enhances data integrity and reduces redundancy in AIoT communication. For instance, integrating network coding into CoAP's block-wise transfer reduces retransmissions in lossy networks [93], while secure network coding schemes like GS-SNC [41] enhance security and efficiency by protecting against attacks.

*2) Bandwidth Optimization Techniques:* Network resource management strategies maximize throughput while minimizing latency across distributed systems [94]. Traffic scheduling prioritizes critical data flows to optimize bandwidth utilization, particularly for real-time applications requiring immediate

response [95]. Rate adaptation, in contrast, dynamically adjusts transmission rates based on network conditions [96]. Specifically, it reduces the rate during congestion and increases it when bandwidth is available. Link aggregation, similarly, combines multiple network links into a single logical link, thereby increasing capacity and resilience against link failures [97]. Notably, this approach enhances efficiency for bandwidth-intensive applications.

*3) Fault Tolerance and Quality Assurance:* Resilient communication infrastructure requires comprehensive error handling and performance monitoring mechanisms [98]. Fault tolerance employs error detection techniques to identify disruptions, data corruption, or device malfunctions, while recovery mechanisms restore functionality through data replication or task rescheduling [87]. Redundancy management, often achieved through redundant hardware or communication paths, ensures data availability and service continuity [52]. Connection management strategies optimize communication performance through link monitoring to identify connectivity issues, failover strategies for seamless transition to backup paths [52], and load balancing to distribute traffic and prevent congestion [95]. In addition, quality assurance practices guarantee reliable service delivery. Specifically, service monitoring tools collect performance data, enabling identification of bottlenecks, while performance optimization techniques, such as bandwidth allocation or data compression, improve efficiency and reduce latency [21, 78]. SLA management ensures that the system meets predefined performance targets. Nonetheless, practices enhance reliability by minimizing errors and reducing latency, the potential trade-off between performance optimization and energy consumption in resource-constrained AIoT environments requires careful consideration [95].

## V. Applications in Smart Cities and Agriculture

### A. Smart Cities

Distributed collaboration significantly enhances the development of intelligent urban environments. Consequently, this collaborative paradigm improves public safety, environmental monitoring, and urban planning within modern networks. For instance, it enhances smart surveillance and crime prevention, leading to improved security and faster response times. In addition, collaborative frameworks contribute to creating more sustainable and livable urban spaces by enabling advanced environmental monitoring and pollution control. They also optimize smart energy management and grid operations, ultimately improving energy efficiency and resource allocation in smart cities.

*1) Smart Surveillance and Crime Prevention:* Real-time security monitoring leverages distributed processing to enhance public safety through intelligent video analytics [53]. Large-scale surveillance data processing benefits from edge deployment of lightweight frameworks such as LISPS, reducing cloud dependency [99]. Additionally, distributing deep learning models, such as A-YONet, which combines YOLO and MTCNN aspects, across the cloud-edge-terminal continuum enhances multi-target detection and activity tracking in complex environments [100]. Furthermore, this collaborative intelligence improves surveillance system efficiency and accuracy while addressing real-time analysis challenges and limited edge computing resources, ultimately facilitating proactive crime prevention through timely suspicious activity identification and efficient resource allocation.

*2) Environmental Monitoring and Pollution Control:* Sustainable urban management requires comprehensive environmental data collection and analysis across distributed sensor networks [78]. City-wide edge devices monitor air quality, water conditions, and noise levels through real-time sensing [23]. Edge computing's localized data processing reduces latency and bandwidth consumption compared to cloud-only solutions [101], enabling faster identification of pollution hotspots and quicker responses to environmental incidents. For complex tasks like predictive modeling and control strategy development, cloud resources are leveraged [21]. For example, machine learning models trained on historical and real-time data can predict future pollution levels, enabling proactive mitigation [46]. Cloud platforms also facilitate data sharing and collaboration among stakeholders, including government agencies, research institutions, and citizens [21].

*3) Smart Energy Management and Grid Optimization:* Grid efficiency improvements emerge through intelligent energy distribution and consumption optimization [102]. Distributed data collection on energy usage and grid conditions informs real-time decision-making for resource allocation [103]. As a result, the collaborative approach facilitates more efficient energy allocation, reducing waste and improving overall grid efficiency. In addition, by analyzing data from various sources, this collaborative paradigm enables predictive maintenance of grid infrastructure, minimizing downtime and improving grid reliability [95]. Integrating renewable energy sources is also supported through this framework [78, 104]. Specifically, edge devices can manage the intermittent nature of renewable energy by intelligently distributing power based on real-time conditions and predicted demand, thereby enhancing grid stability and reducing reliance on fossil fuels.

### B. Smart Agriculture

Distributed collaboration offers transformative potential for intelligent and efficient farming practices. Precision agriculture benefits from real-time data processing and decision-making capabilities provided by collaborative frameworks. Additionally, collaborative systems play a crucial role in crop monitoring and yield prediction by leveraging distributed intelligence to analyze data from diverse sources, including sensors, drones, and satellites. Consequently, this analysis provides insights into crop health, growth patterns, and potential yields, enabling timely interventions and optimized resource allocation for increased agricultural productivity and sustainability.

*1) Precision Agriculture:* Resource optimization in farming benefits from real-time sensor analytics and intelligent decision-making systems [105]. Edge processing of IoT sensor data minimizes latency while enabling immediate responses to changing agricultural conditions [23]. The cloud provides computational power for complex tasks like crop yield prediction and disease detection [60], while federated learning enables distributed model training across farms without sharing

sensitive data, enhancing privacy and model robustness [106]. Consequently, farmers gain actionable insights from real-time data analysis, optimizing resource allocation like water and fertilizer usage, and improving efficiency and sustainability [107]. For example, AI-powered systems analyze sensor data and imagery to detect early signs of crop stress, enabling timely interventions to prevent yield loss [96].

*2) Crop Monitoring and Yield Prediction:* Agricultural intelligence leverages multi-source data integration for enhanced crop management and productivity forecasting. Terminal IoT sensors collect real-time information on soil conditions, weather patterns, and growth stages [108]. Edge devices preprocess and aggregate this data, reducing transmission volume to the cloud and enabling faster localized insights [109]. Accordingly, edge computing facilitates real-time monitoring and control, allowing for prompt responses to changing conditions, such as adjusting irrigation or applying fertilizers based on real-time analysis [110]. The cloud layer, with its extensive computational resources, performs complex analyses, including ML-based yield prediction using historical data, weather forecasts, and real-time sensor data [111, 112]. Furthermore, this information supports farmers' decisions regarding harvesting, resource allocation, and market planning. Cloud-edge collaboration also enables ML model deployment and updates at the edge, adapting models to local conditions and improving accuracy [106]. Moreover, the collaborative approach improves agricultural productivity and promotes sustainable practices by optimizing resource utilization and minimizing environmental impact, such as optimizing harvesting logistics and reducing waste [113, 114].

## References


[1] X. He, H. Xu, X. Xu, Y. Chen, and Z. Wang, "An efficient algorithm for microservice placement in cloud-edge collaborative computing environment," *IEEE Trans. Serv. Comput.*, vol. 17, no. 5, pp. 1983–1997, 2024.

[2] H. Ko, H. Jeong, D. Jung, and S. Pack, "Dynamic split computing framework in distributed serverless edge clouds," *IEEE Internet Things J.*, vol. 11, no. 8, pp. 14 523–14 531, 2024.

[3] N. M. Laboni, S. J. Safa, S. Sharmin, M. A. Razzaque, M. M. Rahman, and M. M. Hassan, "A hyper heuristic algorithm for efficient resource allocation in 5g mobile edge clouds," *IEEE Trans. Mobile Comput.*, vol. 23, no. 1, pp. 29–41, 2024.

[4] Y. Lu, P. Zhang, Y. Duan, M. Guizani, J. Wang, and S. Li, "Dynamic scheduling of iov edge cloud service functions under nfv: A multi-agent reinforcement learning approach," *IEEE Trans. Veh. Technol.*, vol. 73, no. 4, pp. 5730–5741, 2024.

[5] M. D. Nguyen, L. B. Le, and A. Girard, "Integrated computation offloading, uav trajectory control, edge-cloud and radio resource allocation in sagin," *IEEE Trans. Cloud Comput.*, vol. 12, no. 1, pp. 100–115, 2024.

[6] Y. Qiu, J. Liang, V. C. Leung, and M. Chen, "Online security-aware and reliability-guaranteed ai service chains provisioning in edge intelligence cloud," *IEEE Trans. Mobile Comput.*, vol. 23, no. 5, pp. 5933–5948, 2024.

[7] X. Wei, K. Ye, X. Shi, C.-Z. Xu, and Y. Wang, "Joint participant and learning topology selection for federated learning in edge clouds," *IEEE Trans. Parallel Distrib. Syst.*, vol. 35, no. 8, pp. 1456–1468, 2024.

[8] G. Zheng, Q. Ni, K. Navaie, and H. Pervaiz, "Semantic communication in satellite-borne edge cloud network for computation offloading," *IEEE J. Sel. Areas Commun.*, vol. 42, no. 5, pp. 1145–1158, 2024.

[9] M. Asgarian, K. Jamshidi, and A. Bohlooli, "An efficient approximation algorithm for service function chaining placement in edge–cloud computing industrial internet of things," *IEEE Internet Things J.*, vol. 11, no. 7, pp. 12 815–12 822, 2024.

[10] Z. Bai, Y. Lin, Y. Cao, and W. Wang, "Delay-aware cooperative task offloading for multi-uav enabled edge-cloud computing," *IEEE Trans. Mobile Comput.*, vol. 23, no. 2, pp. 1034–1049, 2024.

[11] C. Fang, H. Xu, T. Zhang, Y. Li, W. Ni, Z. Han, and S. Guo, "Joint task offloading and content caching for noma-aided cloud-edge-terminal cooperation networks," *IEEE Trans. Wireless Commun.*, vol. 23, no. 10, pp. 15 586–15 600, 2024.

[12] C. Feng, P. Han, X. Zhang, Q. Zhang, Y. Liu, and L. Guo, "Dependency-aware task reconfiguration and offloading in multi-access edge cloud networks," *IEEE Trans. Mobile Comput.*, vol. 23, no. 10, pp. 9271–9288, 2024.

[13] L. Fu, J. Tong, T. Lin, and J. Zhang, "Data-driven online resource allocation for user experience improvement in mobile edge clouds," *IEEE Trans. Wireless Commun.*, vol. 23, no. 10, pp. 13 707–13 721, 2024.

[14] R.-J. Reifert, H. Dahrouj, and A. Sezgin, "Extended reality via cooperative noma in hybrid cloud/mobile-edge computing networks," *IEEE Internet Things J.*, vol. 11, no. 7, pp. 12 834–12 852, 2024.

[15] H. Xiao, Y. Zhuang, C. Xu, W. Wang, H. Zhang, R. Ding, T. Cao, L. Zhong, and G.-M. Muntean, "Transcoding-enabled cloud–edge–terminal collaborative video caching in heterogeneous iot networks: An online learning approach with time-varying information," *IEEE Internet Things J.*, vol. 11, no. 1, pp. 296–310, 2024.

[16] S. Yue, J. Ren, J. Xin, S. Lin, and J. Zhang, "Inexact-admm based federated meta-learning for fast and continual edge learning," in *MobiHoc*, 2021, pp. 91–100.

[17] T. Zhang, D. Xu, A. Tolba, K. Yu, H. Song, and S. Yu, "Reinforcement-learning-based offloading for ris-aided cloud–edge computing in iot networks: Modeling, analysis, and optimization," *IEEE Internet Things J.*, vol. 11, no. 11, pp. 19 421–19 439, 2024.

[18] K. Zhao, Z. Zhou, L. Jiao, S. Cai, F. Xu, and X. Chen, "Taming serverless cold start of cloud model inference with edge computing," *IEEE Trans. Mobile Comput.*, vol. 23, no. 8, pp. 8111–8128, 2024.

[19] A. Hazra, A. Kalita, and M. Gurusamy, "Distributed

service provisioning with collaboration of edge and cloud in industry 5.0," *IEEE Internet Things J.*, vol. 11, no. 12, pp. 21 885–21 894, 2024.

[20] L. Wu, P. Sun, Z. Wang, Y. Li, and Y. Yang, "Computation offloading in multi-cell networks with collaborative edge-cloud computing: A game theoretic approach," *IEEE Trans. Mobile Comput.*, vol. 23, no. 3, pp. 2093–2106, 2024.

[21] J. Zhou, S. Pal, C. Dong, and K. Wang, "Enhancing quality of service through federated learning in edge-cloud architecture," *Ad Hoc Netw.*, vol. 156, p. 103430, 2024.

[22] G. Dragotto, A. Boukhtouta, A. Lodi, and M. Taobane, "The critical node game," *J. Comb. Optim.*, vol. 47, no. 5, p. 74, 2024.

[23] E. Raj, M. Westerlund, and L. Espinosa-Leal, "Reliable fleet analytics for edge iot solutions," 2021.

[24] X. Gao, R. Liu, and A. Kaushik, "Virtual network function placement in satellite edge computing with a potential game approach," *IEEE Trans. Netw. Service Manag.*, vol. 19, no. 2, pp. 1243–1259, 2022.

[25] Y. Guo, X. Xu, and F. Xiao, "Madrlom: A computation offloading mechanism for software-defined cloud-edge computing power network," *Comput. Netw.*, vol. 245, p. 110352, 2024.

[26] X. Zhang, Z. Wang, F. Tian, and Z. Yang, "Stackelberg-game-based multi-user multi-task offloading in mobile edge computing," *IEEE Trans. Cloud Comput.*, vol. 12, no. 2, pp. 459–475, 2024.

[27] Y. Li, X. Zhang, B. Lei, Q. Zhao, M. Wei, Z. Qu, and W. Wang, "Computation rate maximization for wireless-powered edge computing with multi-user cooperation," *IEEE Open J. Commun. Soc.*, vol. 5, pp. 965–981, 2024.

[28] B. Bandyopadhyay, P. Kuila, M. C. Govil, and M. Bey, "Delay-sensitive task offloading and efficient resource allocation in intelligent edge–cloud environments: A discretized differential evolution-based approach," *Appl. Soft Comput.*, vol. 159, p. 111637, 2024.

[29] C. Zeng, X. Wang, R. Zeng, Y. Li, J. Shi, and M. Huang, "Joint optimization of multi-dimensional resource allocation and task offloading for qoe enhancement in cloud-edge-end collaboration," *Future Gener. Comput. Syst.*, vol. 155, pp. 121–131, 2024.

[30] D. Gan, X. Ge, and Q. Li, "An optimal transport-based federated reinforcement learning approach for resource allocation in cloud–edge collaborative iot," *IEEE Internet Things J.*, vol. 11, no. 2, pp. 2407–2419, 2024.

[31] V. Choudhary, P. Wang, S. Sourav, and B. Chen, "Enhancing data processing throughput in iot-edge-cloud systems using optimized task placement," in *IEEE ICDCS*, 2024, pp. 1474–1475.

[32] K. Khalafi and N. Lu, "Network slicing for edge-cloud orchestrated networks via online convex optimization," in *IEEE INFOCOM*, 2024, pp. 1–6.

[33] X. Chen and S. Zheng, "Resource allocation and task offloading strategy base on hybrid simulated annealing-binary particle swarm optimization in cloud-edge collaborative system," in *IMCEC*, vol. 5, 2022, pp. 379–383.

[34] K. Yu, S. Wang, and X. Tao, "Game theory for 5g cloud-edge-terminal distributed networks under dos attacks," in *IEEE WCNC*, 2024, pp. 1–6.

[35] Y. Duan and C. Jiang, "Binary task offloading strategy for cloud robots using improved game theory in cloud-edge collaboration," *J. Supercomput.*, vol. 80, no. 10, pp. 14 752–14 772, 2024.

[36] F. Shams, V. Lottici, and Z. Tian, "Joint latency-energy minimization for fog-assisted wireless iot networks," *IEEE Open J. Commun. Soc.*, vol. 6, pp. 1–15, 2025.

[37] J. Fang, Y. He, F. R. Yu, J. Li, and V. C. Leung, "Large language models (llms) inference offloading and resource allocation in cloud-edge networks: An active inference approach," in *IEEE VTC*, 2023, pp. 1–5.

[38] A. Zhu, H. Lu, S. Guo, Z. Zeng, M. Ma, and Z. Zhou, "Syroc: Symbiotic robotics for qos-aware heterogeneous applications in iot-edge-cloud computing paradigm," *Future Gener. Comput. Syst.*, vol. 150, pp. 202–219, 2024.

[39] Q. Wang, D. Zhou, and Y. Li, "Secure outsourced calculations with homomorphic encryption," *Adv. Comput. Int. J.*, vol. 9, no. 6, pp. 01–14, 2018.

[40] M. Xiao, Q. Huang, W. Chen, C. Lyu, and W. Susilo, "Domain-specific fine-grained access control for cloud-edge collaborative iot," *IEEE Trans. Inf. Forensics Security*, vol. 19, pp. 6499–6513, 2024.

[41] W. Fang, C. Zhu, and W. Zhang, "Toward secure and lightweight data transmission for cloud–edge–terminal collaboration in artificial intelligence of things," *IEEE Internet Things J.*, vol. 11, no. 1, pp. 105–113, 2024.

[42] C. Chi, Z. Yin, Y. Liu, and S. Chai, "A trusted cloud–edge decision architecture based on blockchain and mlp for aiot," *IEEE Internet Things J.*, vol. 11, no. 1, pp. 201–216, 2024.

[43] Y. Yao, J. Chang, and A. Zhang, "Efficient data sharing scheme with fine-grained access control and integrity auditing in terminal–edge–cloud network," *IEEE Internet Things J.*, vol. 11, no. 16, pp. 26 944–26 954, 2024.

[44] Y. Yigit, C. Chrysoulas, G. Yurdakul, L. Maglaras, and B. Canberk, "Digital twin-empowered smart attack detection system for 6g edge of things networks," in *IEEE GC Wkshps*, 2023, pp. 178–183.

[45] X. Sáez-de-Cámara, J. L. Flores, C. Arellano, A. Urbieta, and U. Zurutuza, "Clustered federated learning architecture for network anomaly detection in large scale heterogeneous iot networks," *Comput. Secur.*, vol. 131, p. 103299, 2023.

[46] Z. Yang, B. Xiong, K. Chen, L. T. Yang, X. Deng, C. Zhu, and Y. He, "Differentially private federated tensor completion for cloud–edge collaborative aiot data prediction," *IEEE Internet Things J.*, vol. 11, no. 1, pp. 256–267, 2024.

[47] Z. Rahman, X. Yi, and I. Khalil, "Blockchain-based ai-enabled industry 4.0 cps protection against advanced persistent threat," *IEEE Internet Things J.*, vol. 10, no. 8, pp. 6769–6778, 2023.

[48] C. Chen, Y. Li, Q. Wang, X. Yang, X. Wang, and L. T. Yang, "An intelligent edge-cloud collaborative framework for communication security in distributed cyber-physical systems," *IEEE Netw.*, vol. 38, no. 1, pp. 172–179, 2024.

[49] Y. Wang, X. Chen, and Q. Wang, "Privacy-preserving security inference towards cloud-edge collaborative using differential privacy," 2022.

[50] M. Wang, J. Santillan, and F. Kuipers, "Thingpot: An interactive internet-of-things honeypot," 2018.

[51] J. Li, L. Lyu, X. Liu, X. Zhang, and X. Lyu, "Fleam: A federated learning empowered architecture to mitigate ddos in industrial iot," *IEEE Trans. Ind. Informat.*, vol. 18, no. 6, pp. 4059–4068, 2022.

[52] H. Dui, J. Wang, T. Zhu, and L. Xing, "Maintenance optimization methodology of edge cloud collaborative systems based on a gateway cost index in iiot," *Reliab. Eng. Syst. Saf.*, vol. 251, p. 110370, 2024.

[53] E. Blasch, R. Xu, Y. Chen, G. Chen, and D. Shen, "Blockchain methods for trusted avionics systems," in *IEEE NAECON*, 2019, pp. 192–199.

[54] T. R. Gadekallu, Q.-V. Pham, D. C. Nguyen, P. K. R. Maddikunta, N. Deepa, B. Prabadevi, P. N. Pathirana, J. Zhao, and W.-J. Hwang, "Blockchain for edge of things: Applications, opportunities, and challenges," *IEEE Internet Things J.*, vol. 9, no. 2, pp. 964–988, 2022.

[55] J. Pan, J. Wang, A. Hester, I. Alqerm, Y. Liu, and Y. Zhao, "Edgechain: An edge-iot framework and prototype based on blockchain and smart contracts," *IEEE Internet Things J.*, vol. 6, no. 3, pp. 4719–4732, 2019.

[56] N. Rodríguez-Barroso, G. Stipcich, D. Jiménez-López, J. A. Ruiz-Millán, E. Martínez-Cámara, G. González-Seco, M. V. Luzón, M. A. Veganzones, and F. Herrera, "Federated learning and differential privacy: Software tools analysis, the sherpa.ai fl framework and methodological guidelines for preserving data privacy," *Inf. Fusion*, vol. 64, pp. 270–292, 2020.

[57] Z. Li, Q. Li, Y. Zhou, W. Zhong, G. Zhang, and C. Wu, "Edge-cloud collaborative learning with federated and centralized features," in *SIGIR*, 2023, pp. 1949–1953.

[58] Y. Liu, P. Huang, F. Yang, K. Huang, and L. Shu, "Quasyncfl: Asynchronous federated learning with quantization for cloud–edge–terminal collaboration enabled aiot," *IEEE Internet Things J.*, vol. 11, no. 1, pp. 59–69, 2024.

[59] Y. Li, S. Yang, X. Ren, and C. Zhao, "Asynchronous federated learning with differential privacy for edge intelligence," 2019.

[60] L. Zhang, X. Wang, J. Wang, R. Pung, H. Wang, and K.-Y. Lam, "An efficient fhe-enabled secure cloud–edge computing architecture for iomt data protection with its application to pandemic modeling," *IEEE Internet Things J.*, vol. 11, no. 9, pp. 15 272–15 284, 2024.

[61] D. Kim, Y. Lee, S. Cheon, H. Choi, J. Lee, H. Youm, D. Lee, and H. Kim, "Privacy set: Privacy-authority-aware compiler for homomorphic encryption on edge-cloud system," *IEEE Internet Things J.*, vol. 11, no. 21, pp. 35 167–35 184, 2024.

[62] Fahina, S. U, Poorna, Supriya, R. M. H, and D. Vasudeva, "Securing the data in cloud using algebra homomorphic encryption scheme based on updated elgamal(ahee)," 2022.

[63] A. Aloufi and P. Hu, "Collaborative homomorphic computation on data encrypted under multiple keys," 2019.

[64] D. Gupta, O. Kayode, S. Bhatt, M. Gupta, and A. S. Tosun, "Hierarchical federated learning based anomaly detection using digital twins for smart healthcare," in *IEEE CIC*, 2021, pp. 16–25.

[65] S. Chatel, C. Knabenhans, A. Pyrgelis, C. Troncoso, and J.-P. Hubaux, "Verifiable encodings for secure homomorphic analytics," 2024.

[66] Y. Zhai, M. Ibrahim, Y. Qiu, F. Boemer, Z. Chen, A. Titov, and A. Lyashevsky, "Accelerating encrypted computing on intel gpus," in *IEEE IPDPS*, 2022, pp. 705–716.

[67] J. Sengupta, S. Ruj, and S. D. Bit, "Sprite: A scalable privacy-preserving and verifiable collaborative learning for industrial iot," in *CCGRID*, 2022, pp. 249–258.

[68] L. Duan, J. Sun, Y. Chen, and M. Gorlatova, "Privascissors: Enhance the privacy of collaborative inference through the lens of mutual information," 2023.

[69] S. Becker, F. Schmidt, A. Gulenko, A. Acker, and O. Kao, "Towards aiops in edge computing environments," in *IEEE BigData*, 2020, pp. 3470–3475.

[70] R. Underwood, J. C. Calhoun, S. Di, and F. Cappello, "Understanding the effectiveness of lossy compression in machine learning training sets," 2024.

[71] H. N. Noura, J. Azar, O. Salman, R. Couturier, and K. Mazouzi, "A deep learning scheme for efficient multimedia iot data compression," *Ad Hoc Netw.*, vol. 138, p. 102998, 2023.

[72] Y. Lu, W. Chen, and H. V. Poor, "User preference aware lossless data compression at the edge," *IEEE Trans. Commun.*, vol. 68, no. 6, pp. 3792–3807, 2020.

[73] F. Taurone, D. E. Lucani, M. Fehér, and Q. Zhang, "Change a bit to save bytes: Compression for floating point time-series data," in *NCC*, 2023, pp. 3756–3761.

[74] O. Shadura, B. P. Bockelman, P. Canal, D. Piparo, and Z. Zhang, "Root i/o compression improvements for hep analysis," *EPJ Web Conf.*, vol. 245, p. 02017, 2020.

[75] T. Melissaris, K. Shaw, and M. Martonosi, "Optimizing iot and web traffic using selective edge compression," 2020.

[76] T. Banerjee, J. Choi, J. Lee, Q. Gong, J. Chen, S. Klasky, A. Rangarajan, and S. Ranka, "Scalable hybrid learning techniques for scientific data compression," 2022.

[77] V. Agrawal, G. Kuldeep, and D. Dey, "Near lossless time series data compression methods using statistics and deviation," in *IEEE GC Wkshps*, 2022, pp. 426–431.

[78] P. Arroba, R. Buyya, R. Cárdenas, J. L. Risco-Martín, and J. M. Moya, "Sustainable edge computing: Challenges and future directions," *Softw. Pract. Exp.*, vol. 54, no. 11, pp. 2272–2296, 2024.

[79] Y. Zheng, Y. Chen, C. Tan, Y. Yang, C. Shu, and L. Chen, "Optimization model for vehicular network data queries in edge environments," *J. Cloud Comput.*, vol. 13, no. 1, p. 145, 2024.

[80] S. Rac and M. Brorsson, "At the edge of a seamless cloud experience," 2021.

[81] D. Antonogiorgakis, A. Britzolakis, P. Chatziadam, A. Dimitriadis, S. Gikas, E. Michalodimitrakis, M. Oikonomakis, N. Siganos, E. Tzagkarakis, Y. Nikoloudakis, S. Panagiotakis, E. Pallis, and E. K. Markakis, "A view on edge caching applications," 2019.

[82] Y. Wang and V. Friderikos, "A survey of deep learning for data caching in edge network," *Informatics*, vol. 7, no. 4, p. 43, 2020.

[83] C. Li, X. Wang, T. Zong, H. Cao, and Y. Liu, "Predictive edge caching through deep mining of sequential patterns in user content retrievals," *Comput. Netw.*, vol. 233, p. 109866, 2023.

[84] H. Torabi, H. Khazaei, and M. Litoiu, "A learning-based caching mechanism for edge content delivery," in *ACM/SPEC ICPE*, 2024, pp. 236–246.

[85] Z. Zhang, M. St-Hilaire, X. Wei, H. Dong, and A. E. Saddik, "How to cache important contents for multi-modal service in dynamic networks: A drl-based caching scheme," *IEEE Trans. Multimedia*, vol. 26, pp. 7372–7385, 2024.

[86] A. Luckow, K. Rattan, and S. Jha, "Pilot-edge: Distributed resource management along the edge-to-cloud continuum," in *IEEE IPDPS*, 2021, pp. 874–878.

[87] A. Javed, K. Heljanko, A. Buda, and K. Främling, "Cefiot: A fault-tolerant iot architecture for edge and cloud," in *IEEE WF-IoT*, 2018, pp. 813–818.

[88] L. Chen, J. Qi, X. Su, and R. Wang, "Remr: A reliability evaluation method for dynamic edge computing network under time constraint," *IEEE Internet Things J.*, vol. 10, no. 5, pp. 4281–4291, 2023.

[89] E. D. Paolo, E. Bassetti, and A. Spognardi, "Security assessment of common open source mqtt brokers and clients," 2023.

[90] C. Gündoğan, C. Amsüss, T. C. Schmidt, and M. Wählisch, "Iot content object security with oscore and ndn: A first experimental comparison," in *IFIP Networking*, 2020, pp. 19–27.

[91] R. Giambona, A. E. C. Redondi, and M. Cesana, "Mqtt+: Enhanced syntax and broker functionalities for data filtering, processing and aggregation," in *ACM Q2SWinet*, 2018, pp. 77–84.

[92] J. Dizdarevic, M. Michalke, and A. Jukan, "Engineering and experimentally benchmarking open source mqtt broker implementations," 2023.

[93] C. V. Phung, J. Dizdarevic, and A. Jukan, "Enhancing block-wise transfer with network coding in coap," in *Euro-ParW*, 2020, pp. 737–741.

[94] S. Li, X. You, S. Zhang, M. Fang, and P. Zhang, "Cloud-edge-device collaborative high concurrency access management for massive iot devices in distribution grid," *IEICE Trans. Fundam. Electron. Commun. Comput. Sci.*, vol. E107.A, no. 7, pp. 946–957, 2024.

[95] F. Wang, X. Wen, L. Li, Y. Wen, S. Zhang, and Y. Liu, "Cloud-edge-end collaborative multi-service resource management for iot-based distribution grid," *IEICE Trans. Fundam. Electron. Commun. Comput. Sci.*, vol. E107.A, no. 9, pp. 1542–1555, 2024.

[96] J. Xu, W. Wan, L. Pan, W. Sun, and Y. Liu, "The fusion of deep reinforcement learning and edge computing for real-time monitoring and control optimization in iot environments," in *EPECE*, 2024, pp. 193–196.

[97] Z. Nezami, K. Zamanifar, K. Djemame, and E. Pournaras, "Decentralized edge-to-cloud load balancing: Service placement for the internet of things," *IEEE Access*, vol. 9, pp. 64 983–65 000, 2021.

[98] J. Nikolić, N. Jubatyrov, and E. Pournaras, "Self-healing dilemmas in distributed systems: Fault correction vs. fault tolerance," *IEEE Trans. Netw. Service Manag.*, vol. 18, no. 3, pp. 2728–2741, 2021.

[99] S. Y. Nikouei, R. Xu, Y. Chen, A. Aved, and E. Blasch, "Decentralized smart surveillance through microservices platform," in *Sens. Syst. Space Appl.*, vol. 11017, 2019, pp. 160–175.

[100] X. Zhou, X. Xu, W. Liang, Z. Zeng, and Z. Yan, "Deep-learning-enhanced multitarget detection for end–edge–cloud surveillance in smart iot," *IEEE Internet Things J.*, vol. 8, no. 16, pp. 12 588–12 596, 2021.

[101] T. Vo, P. Dave, G. Bajpai, and R. Kashef, "Edge, fog, and cloud computing : An overview on challenges and applications," 2022.

[102] X. Zhai, Y. Peng, and X. Guo, "Edge-cloud collaboration for low-latency, low-carbon, and cost-efficient operations," *Comput. Electr. Eng.*, vol. 120, p. 109758, 2024.

[103] W. Hua, P. Liu, and L. Huang, "Energy-efficient resource allocation for heterogeneous edge–cloud computing," *IEEE Internet Things J.*, vol. 11, no. 2, pp. 2808–2818, 2024.

[104] J. Li, Z. Qin, W. Liu, and X. Yu, "Energy-aware and trust-collaboration cross-domain resource allocation algorithm for edge-cloud workflows," *IEEE Internet Things J.*, vol. 11, no. 4, pp. 7249–7264, 2024.

[105] P. Kumar, A. Nelson, Z. Kapetanovic, and R. Chandra, *Affordable Artificial Intelligence – Augmenting Farmer Knowledge with AI*, 2021.

[106] W. Khuen Cheng, J. Cheng Khor, W. Zheng Liew, K. Thye Bea, and Y.-L. Chen, "Integration of federated learning and edge-cloud platform for precision aquaculture," *IEEE Access*, vol. 12, pp. 124 974–124 989, 2024.

[107] F. Z. Bassine, T. E. Epule, A. Kechchour, and A. Chehbouni, "Recent applications of machine learning, remote sensing, and iot approaches in yield prediction: A critical review," 2023.

[108] C. Wang and J. Gong, "Intelligent agricultural greenhouse control system based on internet of things and machine learning," 2025.

[109] Y. Chen, S. Ye, J. Wu, B. Wang, H. Wang, and W. Li, "Fast multi-type resource allocation in local-edge-cloud computing for energy-efficient service provision," *Inf.*

*Sci.*, vol. 668, p. 120502, 2024.

[110] X. Cao, Y. Yao, L. Li, W. Zhang, Z. An, Z. Zhang, L. Xiao, S. Guo, X. Cao, M. Wu, and D. Luo, "igrow: A smart agriculture solution to autonomous greenhouse control," *AAAI*, vol. 36, no. 11, pp. 11 837–11 845, 2022.

[111] F. Huber, A. Yushchenko, B. Stratmann, and V. Steinhage, "Extreme gradient boosting for yield estimation compared with deep learning approaches," *Comput. Electron. Agric.*, vol. 202, p. 107346, 2022.

[112] Z. Cao, Y. Ma, and Z. Zhang, "Corn yield prediction based on remotely sensed variables using variational autoencoder and multiple instance regression," 2022.

[113] H. Chowdhury, D. B. P. Argha, and M. A. Ahmed, "Artificial intelligence in sustainable vertical farming," 2023.

[114] F. Lin, S. Crawford, K. Guillot, Y. Zhang, Y. Chen, X. Yuan, L. Chen, S. Williams, R. Minvielle, X. Xiao, D. Gholson, N. Ashwell, T. Setiyono, B. Tubana, L. Peng, M. Bayoumi, and N.-F. Tzeng, "Mmst-vit: Climate change-aware crop yield prediction via multi-modal spatial-temporal vision transformer," in *ICCV*, 2023, pp. 5774–5784.
